# Supplementary material for: A Combination Framework for Complexity
Source: arXiv:1302.0973 source file (2013-02-05)
Supplement: Supplementary file 1 [file appendix.tex]

\begin{proof}[Proof Of Lemma~\ref{l:rc:monotonecp}]
\end{proof}

%%% Local Variables: 
%%% mode: latex
%%% TeX-master: "paper"
%%% End: 
